# Supplementary material for: Latent-NeRF for Shape-Guided Generation of 3D Shapes and Textures
Source: arXiv:2211.07600 source file (2022-11-14)
Supplement: Supplementary file 2 [file garden_gnomes.tex]

\begin{figure}[h]
    \centering
    \newcommand{\pl}{-4.0}
    \begin{overpic}[width=\columnwidth]{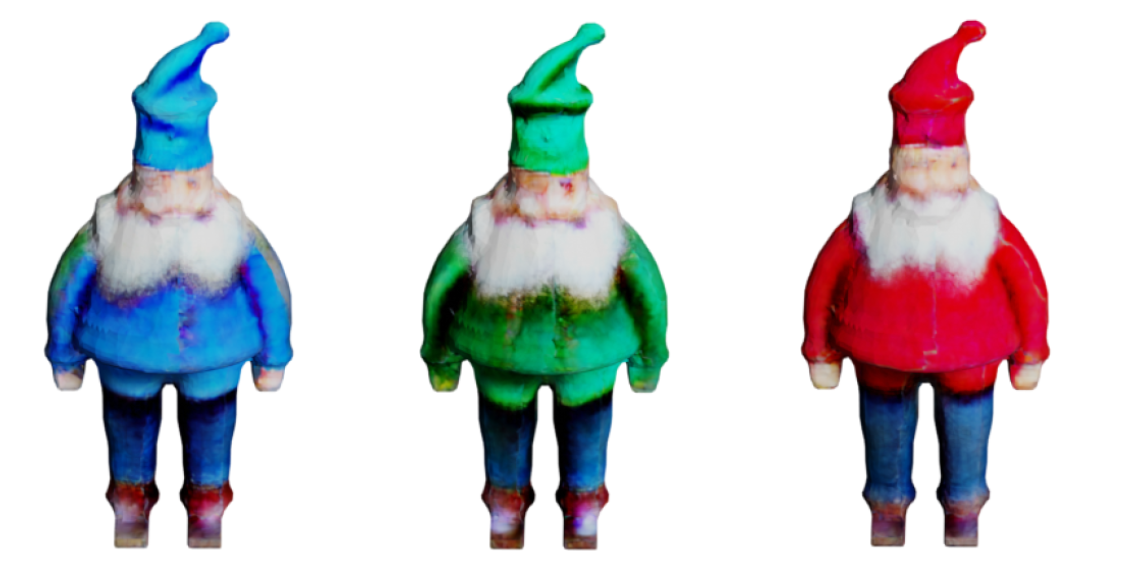}
    \put(71,  \pl){\begin{minipage}{\textwidth}"A garden gnome \\with a red hat"\end{minipage}}
     \put(35,  \pl){\begin{minipage}{\textwidth}"A garden gnome \\with a green hat"\end{minipage}}
    \put(3,  \pl){\begin{minipage}{\textwidth}"A garden gnome \\with a blue hat"\end{minipage}}
    \end{overpic}
    \vspace{1pt}
    \caption{LatnetMesh results over the same input geometry conditioned by different input text prompts.}
    \label{fig:latent_mesh_gnomes}
\end{figure}
