# Supplementary material for: Latent-NeRF for Shape-Guided Generation of 3D Shapes and Textures
Source: arXiv:2211.07600 source file (2022-11-14)
Supplement: Supplementary file 3 [file piano.tex]

\begin{figure}
    \centering
    \begin{overpic}[width=\columnwidth]{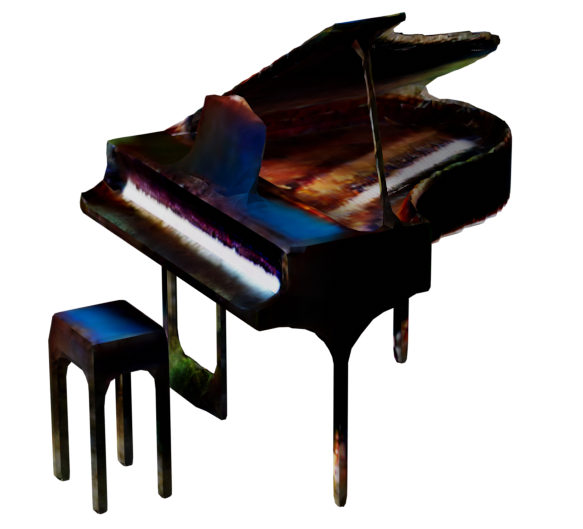}
    \put(30,  0){\begin{minipage}{\textwidth}"A Grand Piano"\end{minipage}}
    \end{overpic}
    \caption{Latent Mesh Colorization of a Grand Piano}
    \label{fig:latnet_mesh_piano}
\end{figure}
